# Supplementary material for: MotiF: Making Text Count in Image Animation with Motion Focal Loss
Source: arXiv:2412.16153 source file (2025-03-23)
Supplement: Supplementary file 1 [file complex_supp.tex]

\begin{figure*}[t]
    \centering
    \includegraphics[width=\linewidth]{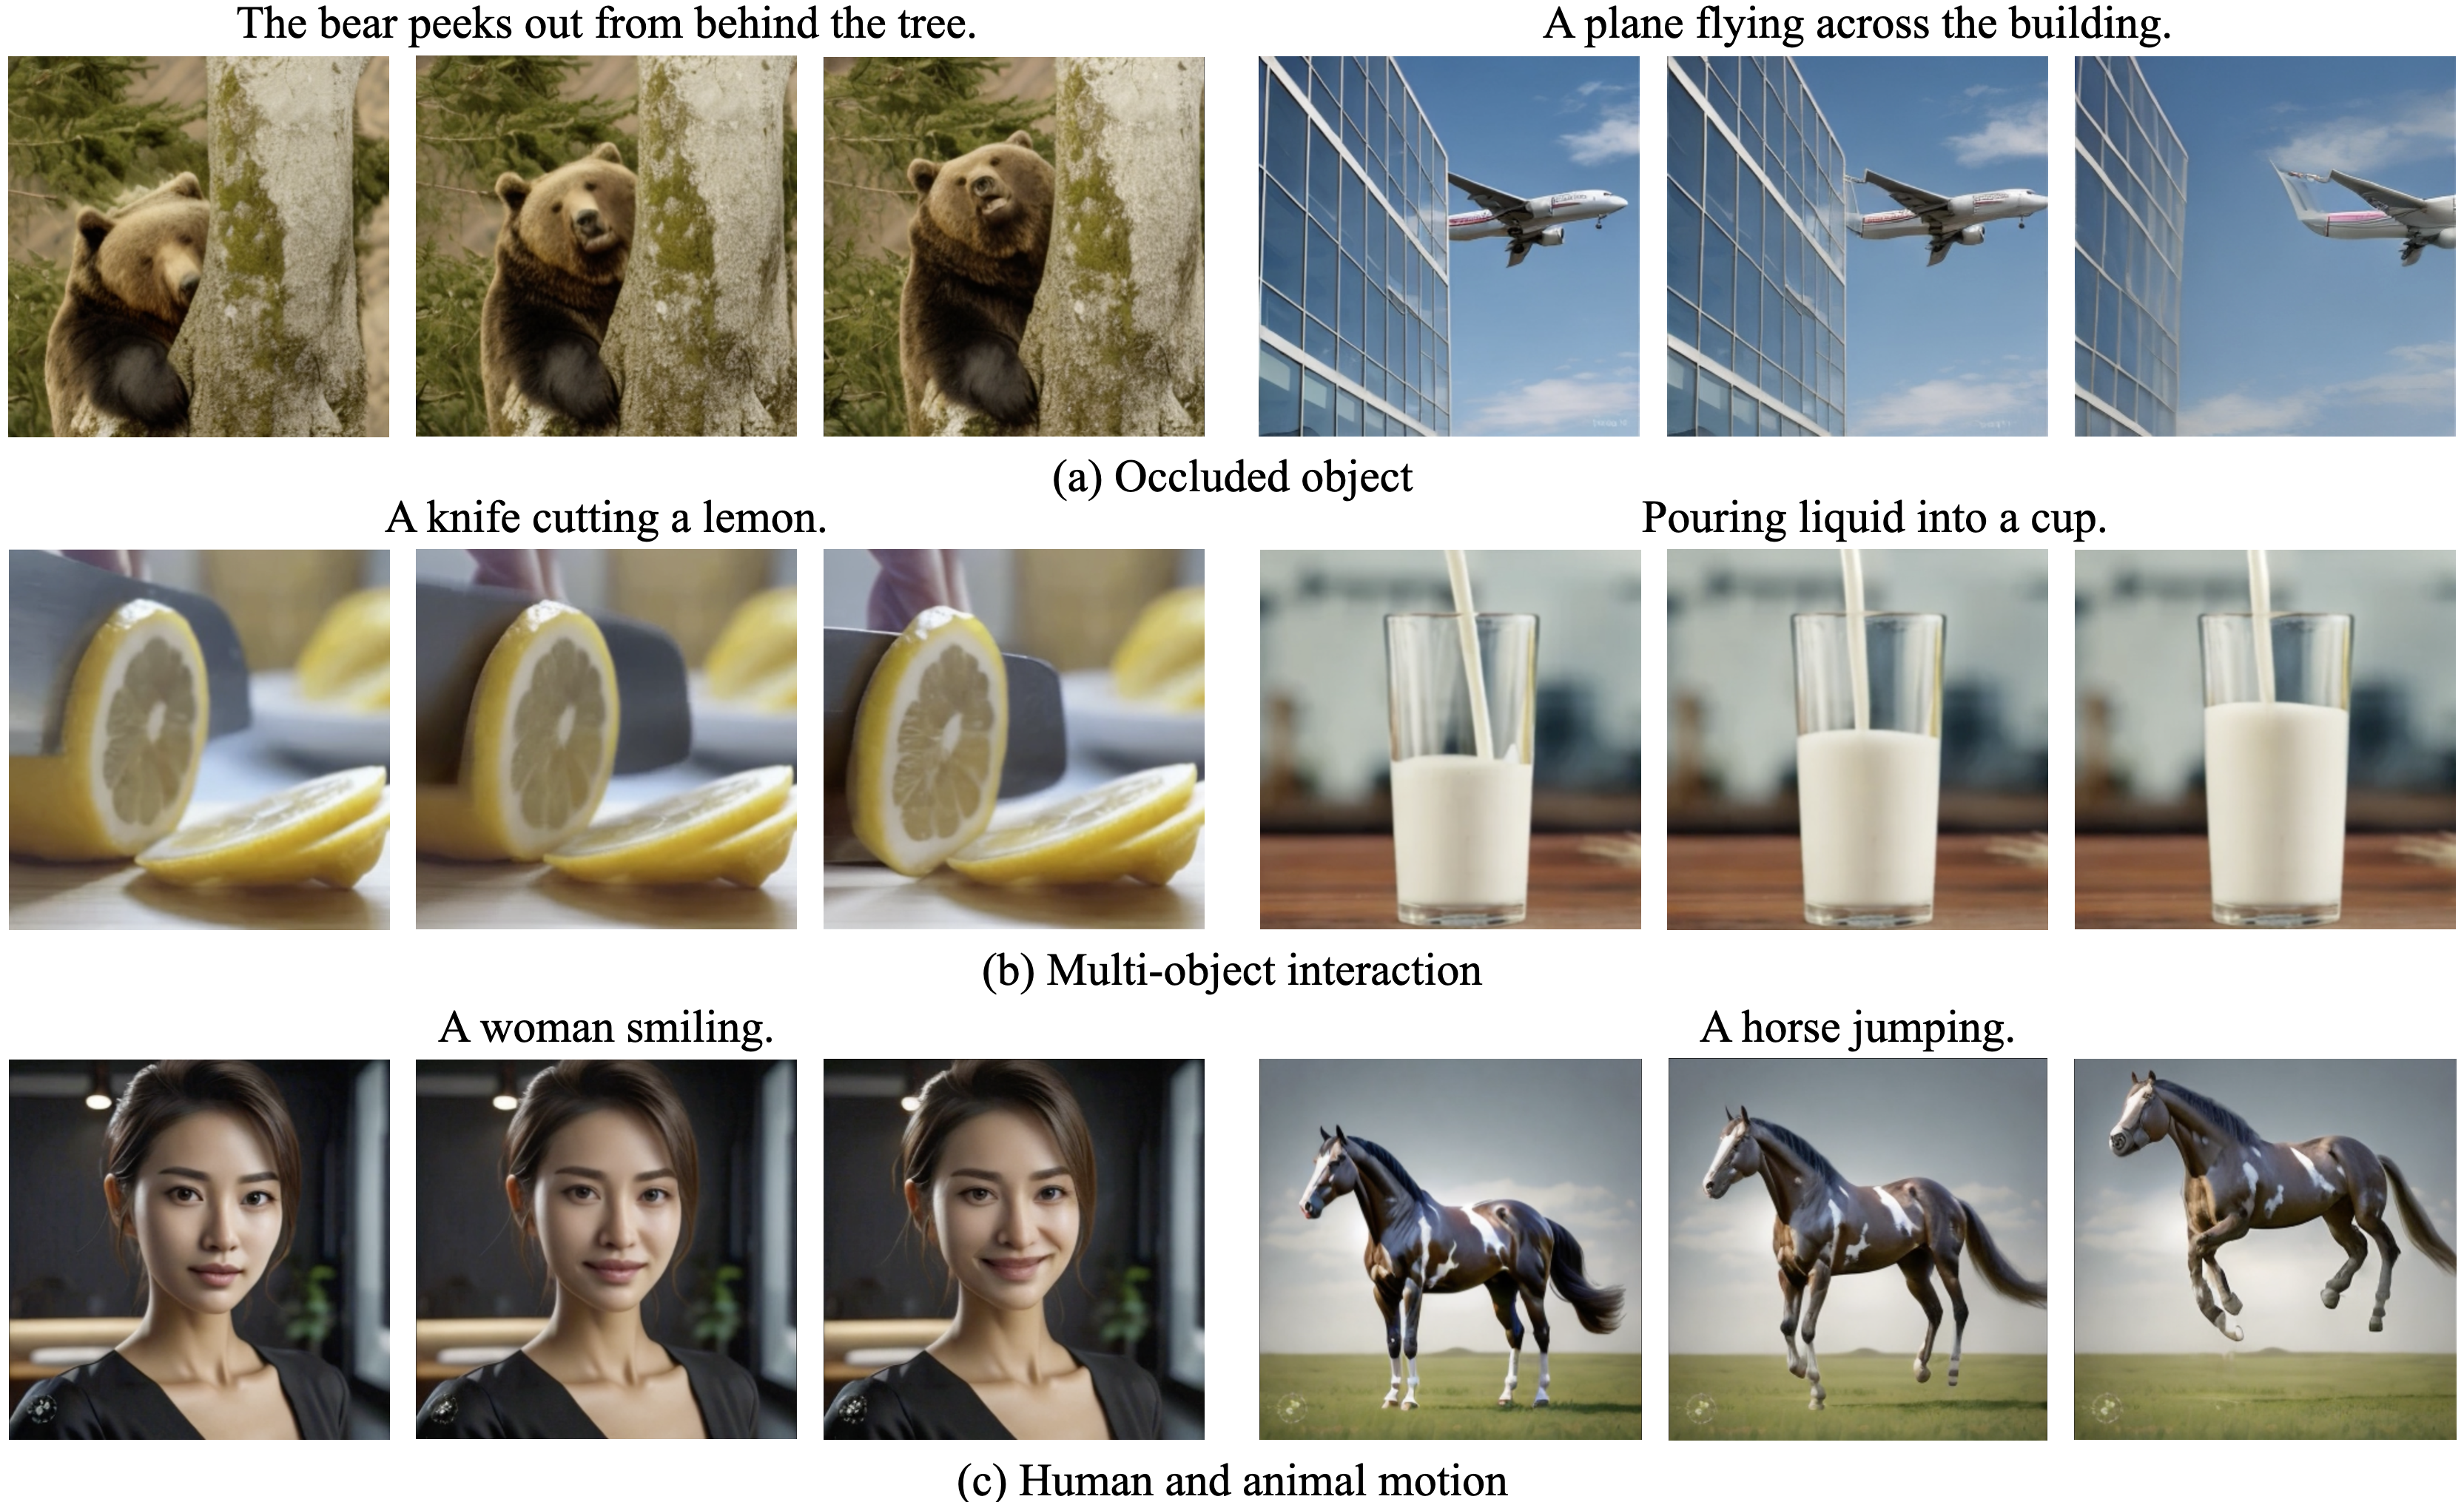}
    \captionof{figure}{\textbf{Results on complex scenarios}}
    \label{fig:complex_supp}
\end{figure*}
